# Supplementary material for: Graphene as Gain Medium for Broadband Lasers
Source: arXiv:1409.8182 source file (2014-09-29)
Supplement: Supplementary file 1 [file graphene_laser_supplementary.pdf]

# Graphene as Gain Medium for Broadband Lasers

# Supplementary Material

Roland Jago, Torben Winzer, Andreas Knorr, and Ermin Malic*

*University of Technology Berlin, Department for Theoretical Physics, Non-linear Optics and Quantum Electronics, Hardenbergstasse 36, 10623 Berlin, Germany*

E-mail: ermin.malic@tu-berlin.de

To obtain microscopic access to the coupled dynamics of electrons, phonons, and photons discussed in the main text, we derive the graphene luminescence equations within the density matrix formalism.[1,2] Applying the correlation expansion and taking into account two-particle processes for electrons and phonons (second-order Born-Markov approximation), we obtain the following set of equations:

$$\dot{\rho}^{\lambda}_{\mathbf{k}}(t) = \Gamma^{in}_{\mathbf{k}\lambda}(t)\left(1-\rho^{\lambda}_{\mathbf{k}}(t)\right) - \Gamma^{out}_{\mathbf{k}\lambda}(t)\,\rho^{\lambda}_{\mathbf{k}}(t) \pm 2\,|\tilde{M}^{vc}_{\mathbf{k}}|^2\,\mathrm{Re}[\,{}^1S^{vc}_{\mathbf{k}}(t)] \pm P(t)\left(\rho^{v}_{\mathbf{k}}(t)-\rho^{c}_{\mathbf{k}}(t)\right) \quad (1)$$

$$\dot{n}^{j}_{\mathbf{q}}(t) = \Gamma^{em}_{\mathbf{q}j}(t)\left(n^{j}_{\mathbf{q}}(t)+1\right) - \Gamma^{abs}_{\mathbf{q}j}(t)\,n^{j}_{\mathbf{q}}(t) - \gamma_{ph}\left(n^{j}_{\mathbf{q}}(t)-n^{j}_{\mathbf{q},B}\right) \quad (2)$$

$$\dot{n}_{pt}(t) = 2\sum_{\mathbf{k}}|\tilde{M}^{vc}_{\mathbf{k}}|^2\,\mathrm{Re}[\,{}^1S^{vc}_{\mathbf{k}}(t)] - 2\kappa\left(n_{pt}(t)-n_B\right), \quad (3)$$

with the pump term $P(t)$ describing the optical excitation of electrons from the valence into the conduction band. The time- and momentum-dependent in- and out-scattering rates $\Gamma^{in/out}_{\mathbf{k}\lambda}(t)$ in Eq. (1) include carrier-carrier and carrier-phonon scattering channels (for more details, see Refs.[3,4]). The carrier-photon interaction leads to additional terms driven by the one-photon-assisted polar-

*To whom correspondence should be addressed

ization ${}^{1}S^{vc}_{\mathbf{k}}(t) = \langle a^{+}_{\mathbf{k}v} a_{\mathbf{k}c} c^{+} \rangle^{c}(t)$. The dynamics of electrons in the conduction ($\lambda = c$) and the valence band ($\lambda = v$) is symmetric ($+$ in Eq. (1) stands for $\lambda = v$ and $-$ for $\lambda = c$). The electronic system is excited by the steady-state-like pumping rate $P(t)$. The dynamics of the phonon number $n^{j}_{\mathbf{q}}$ is driven by the emission and absorption rates $\Gamma^{em/abs}_{\mathbf{q}j}(t)$.[3,4] The temporal evolution of the emitted photons $n_{pt}$ is calculated for the dominant mode $\gamma_0$ determined by the cavity. The phonon and photon lifetimes are denoted by $\gamma_{ph}$ and $\kappa$. The latter is related to the quality factor $Q$ of the cavity via $\kappa = \frac{\omega_0}{2Q}$ with the eigen frequency $\omega_0$. Furthermore, $n^{j}_{\mathbf{q},B}$ and $n_B$ are the initial Bose-distributions for the phonon and photon numbers.

To obtain a closed set of equations, we need to derive an equation of motion for the one-photon assisted polarization ${}^{1}S^{vc}_{\mathbf{k}}(t)$. Assuming that no coherent excitations are allowed, i.e. $\langle c^{+} \rangle = \langle c \ \ \rangle = 0$, and factorizing quantities with four electronic operators, we obtain

$$ {}^{1}\dot{S}^{vc}_{\mathbf{k}}(t) = i\Delta\omega^{vc}_{\mathbf{k}}(t)\ {}^{1}S^{vc}_{\mathbf{k}}(t) + \left(1-\rho^{v}_{\mathbf{k}}(t)\right)\rho^{c}_{\mathbf{k}}(t) - \left(\rho^{v}_{\mathbf{k}}(t)-\rho^{c}_{\mathbf{k}}(t)\right) n_{pt}(t) - {}^{2}S^{vv}_{\mathbf{k}}(t) + {}^{2}S^{cc}_{\mathbf{k}}(t), \quad (4) $$

with $\Delta\omega^{vc}_{\mathbf{k}} = \omega_{\mathbf{k}v} - \omega_{\mathbf{k}c} + \omega_0 + i(\kappa + \gamma_{\mathbf{k}}(t))$. The equation includes the free-particle oscillation and the damping of ${}^{1}S^{vc}_{\mathbf{k}}$ as well as the processes of spontaneous and stimulated emission and absorption of light. The time- and momentum-dependent damping $\gamma_{\mathbf{k}}(t)$ is determined by Coulomb- and phonon-induced scattering processes, which have been explicitly included into the calculations.

The appearing two-photon assisted densities ${}^{2}S^{\lambda\lambda}_{\mathbf{k}} = \langle a^{+}_{\mathbf{k}\lambda} a_{\mathbf{k}\lambda} c^{+} c \ \rangle^{c}(t)$ contain corrections stemming from higher-order many-particle processes.

To characterize the emitted light, we investigate the photon statistics, which is given by the second-order autocorrelation function $g^{(2)}(t)$, cf. Eq. (2) in the main text. Here, quantities including four photonic operators $n_{pt,2}(t) = \langle c^{+} c^{+} c \ \ c \ \rangle^{c}(t)$ appear. Therefore, we have to treat the dynamics of photons up to the forth order in the Born approximation. The equation of motion for

$n_{pt,2}(t)$ reads:

$$\dot{n}_{pt,2}(t) = 4\sum_{\mathbf{k}} |M^{vc}_{\mathbf{k}}|^2\,\mathrm{Re}\big[\,{}^3S^{vc}_{\mathbf{k}}(t)\big] - 4\kappa\, n_{pt,2}(t). \tag{5}$$

The temporal evolution of the three-photon assisted polarization ${}^3S^{vc}_{\mathbf{k}}(t) = \langle a^+_{\mathbf{k}v} a_{\mathbf{k}c} c^+ c^+ c\,\rangle^c(t)$ is given by:

$$\begin{aligned}{}^3\dot{S}^{vc}_{\mathbf{k}}(t) &= i\Big(\omega_{\mathbf{k}v} - \omega_{\mathbf{k}c} + \omega_0 + i\big(3\kappa + \gamma_{\mathbf{k}}(t)\big)\Big)\;{}^3S^{vc}_{\mathbf{k}}(t) \\ &- 2\,|M^{vc}_{\mathbf{k}}|^2\big(\,{}^1S^{vc}_{\mathbf{k}}(t)\big)^2 - \big(\rho^v_{\mathbf{k}}(t) - \rho^c_{\mathbf{k}}(t)\big)n_{pt,2}(t) + 2\,(1-\rho^v_{\mathbf{k}}(t))\;{}^2S^{cc}_{\mathbf{k(t)}} - 2\,\rho^c_{\mathbf{k}}(t)\;{}^2S^{vv}_{\mathbf{k}}(t).\end{aligned} \tag{6}$$

Note that in the equation for ${}^3S^{vc}_{\mathbf{k}}(t)$ as well as in the equation for ${}^1S^{vc}_{\mathbf{k}}(t)$, the two-photon-assisted densities ${}^2S^{\lambda\lambda}_{\mathbf{k}}(t)$ occur, such that they link the photon number to the photon statistics. Their equation of motion reads:

$${}^2\dot{S}^{\lambda\lambda}_{\mathbf{k}}(t) = -\big(2\kappa + \gamma_{\mathbf{k}(t)}\big)\;{}^2S^{\lambda\lambda}_{\mathbf{k}}(t) \pm 2\,|M^{vc}_{\mathbf{k}}|^2\,\mathrm{Re}\big[\,{}^3S^{vc}_{\mathbf{k}}(t) + \big(n_{pt}(t) + 1 - \rho^{\lambda}_{\mathbf{k}}(t)\big)\;{}^1S^{vc}_{\mathbf{k}}(t)\big]. \tag{7}$$

Now, we have a closed set of graphene luminescence equations (1)-(7) allowing us to address the temporally and spectrally resolved dynamics and the quantum statistics of emitted photons from optically pumped graphene within a cavity.

**Carrier recombination rates:** Figure 1 illustrates the temporal evolution of radiative as well as Coulomb-induced and phonon-assisted non-radiative carrier recombination rates after an optical excitation. In graphene on widely used $SiO_2$ or SiC substrates, the Coulomb scattering is the crucial relaxation mechanism that also determines the recombination of excited carrier on a femtosecond timescale.[3,5] The situation changes for graphene on high-dielectric substrates, which strongly suppress the Coulomb interaction. Furthermore, integrating graphene into a nanocavity that enhances the carrier-photon coupling, one can obtain radiative recombination rates that are two orders of magnitude higher than the competing non-radiative processes, cf. Figure 1. This

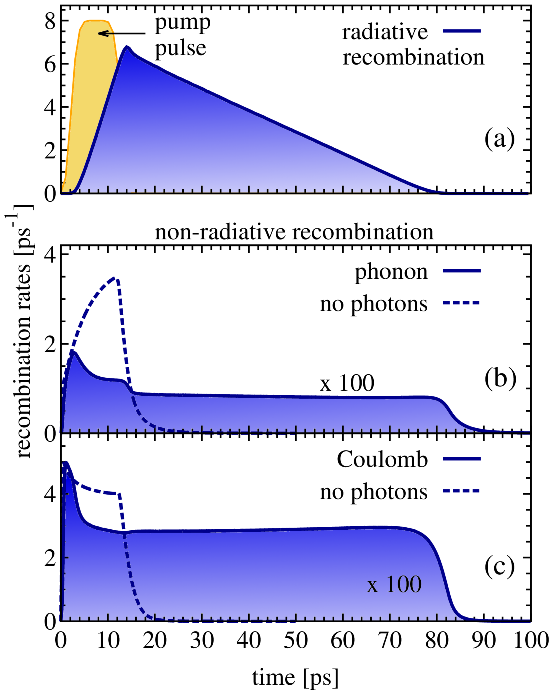


Figure 1: **Radiative and non-radiative recombination rates.** Temporal evolution of (a) radiative, (b) phonon-assisted, and (c) Coulomb-induced non-radiative recombination rates. The corresponding scattering channels are in direct competition with each other during the entire dynamics. Note that the non-radiative recombination rates are two orders of magnitude smaller than the radiative process due to the enhancement of the carrier-light coupling within a nanocavity and due to the suppression of Coulomb interaction through substrate-induced screening. The dashed lines show the rates without taking into account the carrier-photon coupling illustrating the crucial impact of photons on the efficiency of non-radiative recombination channels during and after the optical excitation (displayed by the orange Gaussian-like pump pulse.)

scenario is ideal to obtain a long-lived optical gain that can be used for the amplification of light, as discussed in the main text.

Besides the width of the pulse and the cavity energy discussed in the main text, the pump strength $P_0$ also plays an important role for the coupled carrier, phonon, and photon dynamics. We find a threshold value of approximately $P_0 = 10\,\text{ps}^{-1}$, which is necessary to obtain a population inversion - the prerequisite for pronounced emission of light. The stronger the pumping, the shorter is the delay time in the photon dynamics and the faster is the coherent limit of $g^{(2)} = 1$ reached. Furthermore, the characteristics of the cavity, such as the quality factor $Q$, the volume $V$, and

the cavity energy $\hbar\omega_0$, have an impact on the dynamics. The quality factor $Q$ is a measure for the loss of photons within the cavity. At the considered pumping scenario, values of $Q > 1000$ are already sufficient to reach the laser threshold. The length of the cavity is determined by the considered cavity mode. While the volume of the cavity can be rather large, its size in the direction perpendicular to the graphene layer has a direct impact on the number of emitted photons (Eq. (3) and Eq. (1) from the main text) and has to be in the range of few 100 nm to obtain the emission of coherent laser light. This can be realized even for terahertz frequencies by integrating graphene into planar photonic crystal nanocavities.[6,7]

## References


(1) Kira, M.; Jahnke, F.; Hoyer, W.; Koch, S. *Prog. Quant. Electron.* **1999**, *23*, 189–279.

(2) Gies, C.; Wiersig, J.; Lorke, M.; Jahnke, F. *Phys. Rev. B* **2007**, *75*, 013803.

(3) Malic, E.; Winnerl, S.; Knorr, A. *Graphene and Carbon Nanotubes: Ultrafast Optics and Relaxation Dynamics*; Wiley-VCH, 2013.

(4) Malic, E.; Winzer, T.; Bobkin, E.; Knorr, A. *Phys. Rev. B* **2011**, *84*, 205406.

(5) Winzer, T.; Malić, E.; Knorr, A. *Phys. Rev. B* **2013**, *87*, 165413.

(6) Gan, X.; Mak, K. F.; Gao, Y.; You, Y.; Hatami, F.; Hone, J.; Heinz, T. F.; Englund, D. *Nano Lett.* **2012**, *12*, 5626.

(7) Akahane, Y.; Asano, T.; Song, B. S.; Noda, S. *Nature* **2003**, *425*, 944.
